# Supplementary material for: Data-Adaptive Mahalanobis Metric Learning for Cross-Head Attention in Transformers
Source: arXiv:2610.13261 source file (2026-10-09)
Supplement: Supplementary file 1 [file damcha_theory_supplement.tex]

% --------------------------------------------------------
%  3.2  Data-Adaptive Cross-Head Metric Learning
% --------------------------------------------------------
\subsection{Data-Adaptive Cross-Head Metric Learning}

In standard MHA, each head metric $M_{i,i}$ is fixed after
training, which implies that the same projection matrices are
applied to all inputs $X$ during inference.
Although attention scores $XM_{i,i}X^\top$ vary with the input
contents, the underlying metric $M_{i,i}$ itself is
input-independent.
In other words, MHA learns a static metric that is globally shared
across all contexts.
This static design may be suboptimal in practice: the relevance
between two features may be strong in one context but weak in
another, yet a fixed metric cannot adapt its attention geometry
accordingly.

To increase the expressiveness of the attention mechanism, we
parameterize CHM as an \emph{input-dependent} function.
Concretely, a learnable forward network $f_\theta(\cdot)$ (e.g.,
an MLP or a hyper-network) is introduced to generate the
\emph{diagonal} blocks of the CHM conditioned on the input:
\begin{equation}
f_\theta(X)
\;\longrightarrow\;
\bigl(M_{1,1}(X),\,M_{2,2}(X),\,\ldots,\,M_{h,h}(X)\bigr).
\label{eq:diag-generator-main}
\end{equation}
Under this formulation, each diagonal block $M_{k,k}(X)$ is no
longer a matrix with constant parameters, but is dynamically
generated conditioned on the input $X$.
This allows the model to dynamically select appropriate geometries
for different contexts, aligning the attention operator with the
local structure of the data manifold.

To model cross-head interactions while controlling parameter
cost, we impose a \emph{linear structural constraint} on the
off-diagonal blocks: each $M_{i,j}(X)$ with $i\neq j$ is
expressed as a linear combination of the diagonal blocks:
\begin{equation}
M_{i,j}(X)
=
\sum_{k=1}^{h}\alpha_{k}^{(i,j)}\,M_{k,k}(X),
\qquad i\neq j,
\label{eq:offdiag-constraint-main}
\end{equation}
where $\alpha_{k}^{(i,j)}\in\mathbb{R}$ are learnable scalar
coefficients (shared across inputs and across layers under
stack-wise sharing).
This setting significantly reduces the effective degrees of
freedom: $f_\theta$ only needs to generate $h$ diagonal blocks,
while all off-diagonal interactions are expressed as weighted
mixtures of these primary subspace metrics.
The constraint also introduces an inductive bias that cross-head
interactions are semantically grounded in the primary feature
subspaces, ensuring that the resulting high-rank attention pattern
remains contextually coherent and structurally regularized.

The full CHM is therefore determined by the diagonal blocks
produced by $f_\theta$ together with the learnable coefficients
$\{\alpha_k^{(i,j)}\}$:
\begin{equation}
M(X) =
\begin{pmatrix}
M_{1,1}(X) & \cdots & M_{1,h}(X) \\
\vdots  & \ddots & \vdots  \\
M_{h,1}(X) & \cdots & M_{h,h}(X)
\end{pmatrix},
\label{eq:full-chm-main}
\end{equation}
where $M_{i,j}(X)$ for $i\neq j$ is given by
\eqref{eq:offdiag-constraint-main}.
Further discussion of the expressive advantages of this
formulation is provided in Appendix~\ref{app:Appendix A}.


% --------------------------------------------------------
%  3.3  Attention Computation
% --------------------------------------------------------
\subsection{Attention Computation}

For head $i$, DAMCHA first computes the \emph{row-summed head
metric} by summing the $i$-th row of the CHM:
\begin{equation}
m_i(X)
=
\sum_{j=1}^{h}M_{i,j}(X).
\label{eq:row-sum-main}
\end{equation}
Substituting constraint~\eqref{eq:offdiag-constraint-main} and
defining the effective mixing coefficients
\begin{equation}
\tilde{\beta}_{i,k}
:=
\delta_{ik}+\sum_{j\neq i}\alpha_{k}^{(i,j)},
\label{eq:beta-tilde-main}
\end{equation}
where $\delta_{ik}$ is the Kronecker delta, we obtain
\begin{equation}
m_i(X) = \sum_{k=1}^{h}\tilde{\beta}_{i,k}\,M_{k,k}(X).
\label{eq:effective-mi-main}
\end{equation}
The pre-softmax score of head $i$ is computed via a generalized
quadratic form:
\begin{equation}
S_i^{\mathrm{DAMCHA}}(X)
=
\frac{1}{\sqrt{d_h}}
X_i\,m_i(X)\,X_i^\top
\in\mathbb{R}^{L\times L}.
\label{eq:damcha-score-main}
\end{equation}
The attention matrix is obtained by row-wise softmax:
\begin{equation}
A_i(X)
=
\operatorname{Softmax}\!\bigl(S_i^{\mathrm{DAMCHA}}(X)\bigr).
\end{equation}
The value representation and head output are
\begin{equation}
V_i=XW_V^{(i)},\quad
W_V^{(i)}\in\mathbb{R}^{d_{\mathrm{model}}\times d_v},
\qquad
O_i(X)=A_i(X)V_i.
\end{equation}
The outputs of all heads are concatenated and projected back:
\begin{equation}
X'
=
\operatorname{Concat}\!\bigl(O_1(X),\ldots,O_h(X)\bigr)\,W_O,
\qquad
W_O\in\mathbb{R}^{(hd_v)\times d_{\mathrm{model}}}.
\end{equation}
Thus, DAMCHA differs from standard MHA primarily in the formation
of pre-softmax attention scores; the value projections and output
projection retain the standard multi-head attention structure.
The workflow of DAMCHA and its difference from MHA are illustrated
in Figure~\ref{workflow}.


% --------------------------------------------------------
%  3.4  Constrained DAMCHA and Its Relation to MHA
% --------------------------------------------------------
\subsection{Constrained DAMCHA and Its Relation to MHA}

The next proposition makes explicit how each attention score is
formed from the diagonal metric blocks shared across heads.

\begin{proposition}[Cross-head metric-basis mixing]
\label{prop:metric-basis-mixing}
Let $M_{k,k}(X)\in\mathbb{R}^{d_h\times d_h}$ ($k=1,\ldots,h$) be
the data-adaptive diagonal blocks generated by $f_\theta$, and let
$\tilde{\beta}_{i,k}$ be the effective coefficients defined in
\eqref{eq:beta-tilde-main}.
Then the pre-softmax score of head $i$ satisfies
\begin{equation}
S_i^{\mathrm{DAMCHA}}(X)
=
\frac{1}{\sqrt{d_h}}
\sum_{k=1}^{h}
\tilde{\beta}_{i,k}\,
X_i M_{k,k}(X) X_i^\top.
\label{eq:basis-score-decomp-main}
\end{equation}
Hence each head forms its attention geometry as a weighted mixture
of score matrices induced by the shared diagonal metric blocks,
where the weight $\tilde{\beta}_{i,i}=1+\sum_{j\neq i}\alpha_i^{(i,j)}$
controls the self-contribution and $\tilde{\beta}_{i,k}=\sum_{j\neq i}\alpha_k^{(i,j)}$
($k\neq i$) controls the cross-head contribution.
\end{proposition}

The proof of Proposition~\ref{prop:metric-basis-mixing} is provided
in Appendix~\ref{app:proof-metric-basis-mixing}.

The following result clarifies the precise sense in which standard
MHA is contained in constrained DAMCHA.

\begin{lemma}[MHA as a degenerate case of constrained DAMCHA]
\label{lem:mha-degenerate}
Standard MHA is recovered from constrained DAMCHA under the
following two restrictions:
\begin{enumerate}
    \item[(C1)] All off-diagonal mixing coefficients vanish:
    \[
    \alpha_{k}^{(i,j)}=0
    \quad\text{for all }i\neq j,\;k=1,\ldots,h;
    \]
    \item[(C2)] The metric generator $f_\theta$ is restricted to a
    constant (input-independent) mapping with each diagonal block
    equal to the corresponding MHA query--key metric:
    \[
    M_{i,i}(X)\equiv\bar{M}_{i,i}
    =
    U_Q^{(i)}\bigl(U_K^{(i)}\bigr)^\top,
    \]
    where $U_Q^{(i)},U_K^{(i)}\in\mathbb{R}^{d_h\times d_h}$ are
    the within-head query and key projections.
\end{enumerate}
Under (C1)--(C2), the pre-softmax score, attention matrix, head
output, and final output of constrained DAMCHA coincide with those
of standard MHA.
\end{lemma}

The proof of Lemma~\ref{lem:mha-degenerate} is provided in
Appendix~\ref{app:proof-mha-degenerate}.

Lemma~\ref{lem:mha-degenerate} establishes that removing cross-head
metric mixing ((C1)) and input-adaptive metric generation ((C2))
recovers standard MHA exactly.
Conversely, whenever some $\alpha_k^{(i,j)}\neq 0$, constrained
DAMCHA relaxes the independent-head scoring restriction of standard
MHA.

\begin{corollary}[Relaxation of independent-head scoring]
\label{cor:independent-head-relaxation}
Constrained DAMCHA relaxes the independent-head scoring restriction
of standard MHA.  If there exist $i\neq j$ and some $k$ such that
$\alpha_{k}^{(i,j)}\neq 0$, then $\tilde{\beta}_{i,k}\neq\delta_{ik}$,
and the score of head $i$ depends on $M_{k,k}(X)$, which is not
exclusively assigned to head $i$.
\end{corollary}

The proof of Corollary~\ref{cor:independent-head-relaxation} is
provided in Appendix~\ref{app:proof-independent-head-relaxation}.

It is also noted that, by allowing all $M_{i,j}(X)$ to be freely
learned without rank restrictions (through the diagonal blocks that
are unconstrained in rank), DAMCHA effectively alleviates the
low-rank bottleneck inherent in conventional attention mechanisms.


% --------------------------------------------------------
%  3.5  Bilinear Similarity Without PSD Constraint
% --------------------------------------------------------
\subsection{Bilinear Similarity Without PSD Constraint}

Although DAMCHA is motivated from a metric-learning perspective,
the learned matrices are not required to be positive semi-definite.
This is because attention uses the resulting quantities as
real-valued pre-softmax logits, rather than as squared distances.

\begin{proposition}[Validity of generalized bilinear similarity]
\label{prop:generalized-bilinear}
Let $x_a,x_b\in\mathbb{R}^{d_h}$ be two token representations and
let $M\in\mathbb{R}^{d_h\times d_h}$ be an arbitrary real-valued
matrix.  The compatibility score $s_{ab}=x_a^\top Mx_b$ defines a
valid pre-softmax attention logit.  Therefore, $M$ does not need to
be positive semi-definite for attention-score formation.
\end{proposition}

The proof of Proposition~\ref{prop:generalized-bilinear} is provided
in Appendix~\ref{app:proof-generalized-bilinear}.

Accordingly, DAMCHA should be interpreted as learning generalized
Mahalanobis-type bilinear similarities for attention logits, rather
than strict Mahalanobis distance metrics.


% --------------------------------------------------------
%  3.6  Function-Class Hierarchy and Approximation Consequence
% --------------------------------------------------------
\subsection{Function-Class Hierarchy and Approximation Consequence}

We next formalize the relation among standard MHA, constrained
DAMCHA, and the unconstrained conceptual CHM.
Let $\mathcal{X}$ be the input domain and $\mathcal{Y}$ a normed
linear space containing score matrices.
For a target score mapping $S^\star:\mathcal{X}\to\mathcal{Y}$,
define the worst-case approximation error of a score class
$\mathcal{S}$ as
\begin{equation}
\varepsilon(\mathcal{S};S^\star)
:=
\inf_{S\in\mathcal{S}}
\sup_{X\in\mathcal{X}}
\|S(X)-S^\star(X)\|_{\mathcal{Y}}.
\label{eq:approx-error-main}
\end{equation}
Let $\mathcal{S}_{\mathrm{MHA}}$, $\mathcal{S}_{\mathrm{cDAM}}$,
and $\mathcal{S}_{\mathrm{uDAM}}$ denote the score-mapping classes
realized by standard MHA, constrained DAMCHA, and unconstrained
DAMCHA, respectively.

\begin{proposition}[Function-class hierarchy]
\label{prop:function-class-hierarchy}
The three score-mapping classes satisfy
\begin{equation}
\mathcal{S}_{\mathrm{MHA}}
\subseteq
\mathcal{S}_{\mathrm{cDAM}}
\subseteq
\mathcal{S}_{\mathrm{uDAM}}.
\label{eq:class-inclusion-main}
\end{equation}
\end{proposition}

The proof of Proposition~\ref{prop:function-class-hierarchy} is
provided in Appendix~\ref{app:proof-function-class-hierarchy}.

\begin{corollary}[Approximation consequence]
\label{cor:approx-consequence}
For any target score mapping $S^\star:\mathcal{X}\to\mathcal{Y}$,
\begin{equation}
\varepsilon(\mathcal{S}_{\mathrm{uDAM}};S^\star)
\le
\varepsilon(\mathcal{S}_{\mathrm{cDAM}};S^\star)
\le
\varepsilon(\mathcal{S}_{\mathrm{MHA}};S^\star).
\label{eq:approx-chain-main}
\end{equation}
\end{corollary}

The proof of Corollary~\ref{cor:approx-consequence} is provided in
Appendix~\ref{app:proof-approx-consequence}.

This approximation consequence is a function-class statement.
It does not claim that DAMCHA always improves optimization or
generalization under finite data, finite training budgets, or a
particular regularization scheme.
Rather, it clarifies that constrained DAMCHA contains standard MHA
as a special case while remaining a structured subset of the
unconstrained CHM formulation.


% --------------------------------------------------------
%  3.7  Metric-Parameter Complexity
% --------------------------------------------------------
\subsection{Metric-Parameter Complexity}

The unconstrained CHM contains $h^2$ metric blocks
$M_{i,j}\in\mathbb{R}^{d_h\times d_h}$, yielding metric-parameter
complexity $O(h^2d_h^2)$.
In constrained DAMCHA, $f_\theta$ generates only the $h$ diagonal
blocks ($hd_h^2$ parameters), and off-diagonal interactions are
controlled by the static scalar coefficients $\alpha_k^{(i,j)}$.
There are $h(h-1)$ ordered off-diagonal pairs, each requiring $h$
scalars, contributing $h^2(h-1)$ parameters.
The total metric-parameter complexity is therefore
$O(hd_h^2+h^3)$.

\begin{proposition}[Metric-parameter complexity]
\label{prop:metric-parameter-complexity}
Let $h$ be the number of heads and $d_h$ be the hidden dimension
per head.
The unconstrained CHM has metric-parameter complexity
$O(h^2d_h^2)$, whereas constrained DAMCHA has metric-parameter
complexity $O(hd_h^2+h^3)$.
Since $d_h\gg h$ in typical architectures, the dominant cost
in both cases is determined by the $d_h^2$ factor, confirming that
constrained DAMCHA achieves substantial parameter savings over the
unconstrained formulation.
\end{proposition}

The proof of Proposition~\ref{prop:metric-parameter-complexity} is
provided in Appendix~\ref{app:proof-metric-parameter-complexity}.

This comparison concerns the number of free parameters used to
represent the cross-head metric structure.
It should not be interpreted as a full runtime complexity bound
for the entire attention layer, since runtime also depends on
sequence length, matrix multiplication kernels, and implementation
details.


% --------------------------------------------------------
%  3.8  Stack-Wise Sharing
% --------------------------------------------------------
\subsection{Stack-Wise Sharing}

In practical Transformer architectures, attention modules are
stacked across multiple layers.
Assigning an independent metric-generating network $f_\theta$ to
each layer would substantially increase the number of parameters
and may lead to overfitting.
Therefore, DAMCHA adopts a \emph{stack-wise sharing} strategy:
all layers reuse the same $f_\theta$ while applying it to
layer-specific hidden representations.
The learnable coefficients $\{\alpha_k^{(i,j)}\}$ are likewise
shared globally across layers.

For the $\ell$-th layer with hidden representation $X^{(\ell)}$,
the shared network generates the adaptive diagonal blocks:
\begin{equation}
\bigl(M_{1,1}^{(\ell)},\ldots,M_{h,h}^{(\ell)}\bigr)
=
f_\theta\!\bigl(X^{(\ell)}\bigr),
\end{equation}
where $\theta$ is shared across layers.
Off-diagonal blocks are then formed via
\eqref{eq:offdiag-constraint-main}, and the attention update is
\begin{equation}
X^{(\ell+1)}
=
\operatorname{DAMCHA}\!\bigl(
X^{(\ell)};\,f_\theta,\,\{\alpha_k^{(i,j)}\}
\bigr).
\end{equation}

This design reduces parameter growth when the number of layers
increases and acts as a regularizer by encouraging different layers
to reuse a consistent family of metric transformations.
Empirically, we observe that this shared design improves training
stability in deep architectures.


% ============================================================
%  APPENDIX --- Proofs
% ============================================================
% (以下放入对应的 \section{...} 或 \subsection{...} 结构中)




% --------------------------------------------------------
%  Proof of Proposition~\ref{prop:metric-basis-mixing}
% --------------------------------------------------------
\subsection{Proof of Proposition~\ref{prop:metric-basis-mixing}}
\label{app:proof-metric-basis-mixing}

\begin{proof}
For head $i$, the row-summed metric is
$m_i(X)=\sum_{j=1}^{h}M_{i,j}(X)$.
Separating diagonal and off-diagonal terms and applying
constraint~\eqref{eq:offdiag-constraint-main}:
\begin{align}
m_i(X)
&=
M_{i,i}(X)
+\sum_{j\neq i}\sum_{k=1}^{h}\alpha_{k}^{(i,j)}M_{k,k}(X) \\
&=
\sum_{k=1}^{h}
\!\Bigl(\delta_{ik}+\textstyle\sum_{j\neq i}\alpha_{k}^{(i,j)}\Bigr)
M_{k,k}(X)
\;=\;
\sum_{k=1}^{h}\tilde{\beta}_{i,k}\,M_{k,k}(X).
\end{align}
Substituting into the DAMCHA score and using linearity of matrix
multiplication in the middle factor:
\[
S_i^{\mathrm{DAMCHA}}(X)
=
\frac{1}{\sqrt{d_h}}X_i m_i(X)X_i^\top
=
\frac{1}{\sqrt{d_h}}
\sum_{k=1}^{h}
\tilde{\beta}_{i,k}\,X_i M_{k,k}(X)X_i^\top.
\qedhere
\]
\end{proof}


% --------------------------------------------------------
%  Proof of Lemma~\ref{lem:mha-degenerate}
% --------------------------------------------------------
\subsection{Proof of Lemma~\ref{lem:mha-degenerate}}
\label{app:proof-mha-degenerate}

\begin{proof}
Under (C1), $\alpha_k^{(i,j)}=0$ for all $i\neq j$ and all $k$,
so $\tilde{\beta}_{i,k}=\delta_{ik}$ and
$m_i(X)=M_{i,i}(X)$.
Under (C2), $M_{i,i}(X)\equiv U_Q^{(i)}(U_K^{(i)})^\top$.
Therefore:
\begin{align}
S_i^{\mathrm{cDAM}}(X)
&=
\frac{1}{\sqrt{d_h}}X_i M_{i,i}(X)X_i^\top
=
\frac{1}{\sqrt{d_h}}X_i U_Q^{(i)}\bigl(U_K^{(i)}\bigr)^\top X_i^\top
=
S_i^{\mathrm{MHA}}(X).
\end{align}
Since both mechanisms apply the same row-wise softmax, their
attention matrices coincide:
$A_i^{\mathrm{cDAM}}(X)=A_i^{\mathrm{MHA}}(X)$.
With the same value projection $W_V^{(i)}$ and output projection
$W_O$, it follows that
$O_i^{\mathrm{cDAM}}(X)=O_i^{\mathrm{MHA}}(X)$,
$O_{\mathrm{cat}}^{\mathrm{cDAM}}(X)=O_{\mathrm{cat}}^{\mathrm{MHA}}(X)$,
and $X_{\mathrm{cDAM}}'=X_{\mathrm{MHA}}'$.
\end{proof}


% --------------------------------------------------------
%  Proof of Corollary~\ref{cor:independent-head-relaxation}
% --------------------------------------------------------
\subsection{Proof of Corollary~\ref{cor:independent-head-relaxation}}
\label{app:proof-independent-head-relaxation}

\begin{proof}
In standard MHA, the score of head $i$ depends only on
$M_{i,i}=U_Q^{(i)}(U_K^{(i)})^\top$, exclusively assigned to
head $i$.

In constrained DAMCHA, if there exist $i\neq j$ and some $k$ such
that $\alpha_k^{(i,j)}\neq 0$, then
$\tilde{\beta}_{i,k}=\delta_{ik}+\sum_{j'\neq i}\alpha_k^{(i,j')}\neq\delta_{ik}$.
Hence the term $\tilde{\beta}_{i,k}\,X_i M_{k,k}(X)X_i^\top$
contributes to $S_i^{\mathrm{DAMCHA}}(X)$ for some $k\neq i$,
meaning the score of head $i$ depends on $M_{k,k}(X)$, which is
not exclusively assigned to head $i$.
This proves that constrained DAMCHA relaxes the independent-head
scoring restriction of standard MHA.
\end{proof}


% --------------------------------------------------------
%  Proof of Proposition~\ref{prop:generalized-bilinear}
% --------------------------------------------------------
\subsection{Proof of Proposition~\ref{prop:generalized-bilinear}}
\label{app:proof-generalized-bilinear}

\begin{proof}
The attention weight $A_{ab}=\exp(s_{ab})/\sum_c\exp(s_{ac})$ is
well-defined for any real-valued logits $s_{ab}$.
The softmax does not require logits to be non-negative, symmetric,
or induced by a positive semi-definite matrix.
A PSD constraint would be necessary only if $x^\top Mx$ were used
as a squared Mahalanobis distance; DAMCHA uses it as a
query--key compatibility logit, so no PSD requirement applies.
Moreover, the skew-symmetric component
$M_{\mathrm{skew}}=\tfrac{1}{2}(M-M^\top)$ satisfies
$x_a^\top M_{\mathrm{skew}}x_b=-x_b^\top M_{\mathrm{skew}}x_a$,
encoding directional compatibility that a strict PSD constraint
would eliminate.
\end{proof}


% --------------------------------------------------------
%  Proof of Proposition~\ref{prop:function-class-hierarchy}
% --------------------------------------------------------
\subsection{Proof of Proposition~\ref{prop:function-class-hierarchy}}
\label{app:proof-function-class-hierarchy}

\begin{proof}
\textbf{Step~1: $\mathcal{S}_{\mathrm{MHA}}\subseteq\mathcal{S}_{\mathrm{cDAM}}$.}
Take any $S\in\mathcal{S}_{\mathrm{MHA}}$.
Construct a constrained DAMCHA parameterization by setting
$\alpha_k^{(i,j)}=0$ for all $i\neq j,k$, and
$M_{i,i}(X)\equiv U_Q^{(i)}(U_K^{(i)})^\top$.
Then $\tilde{\beta}_{i,k}=\delta_{ik}$ and
$S_i^{\mathrm{cDAM}}(X)=S_i(X)$ for every head $i$,
so every MHA score mapping is realizable by constrained DAMCHA.

\textbf{Step~2: $\mathcal{S}_{\mathrm{cDAM}}\subseteq\mathcal{S}_{\mathrm{uDAM}}$.}
Take any $S\in\mathcal{S}_{\mathrm{cDAM}}$.
In the unconstrained DAMCHA class, set
$M_{i,j}(X):=\sum_k\alpha_k^{(i,j)}M_{k,k}(X)$ for $i\neq j$
(using the same coefficients).
Then the unconstrained row-sum recovers $m_i(X)$ exactly, so the
same score mapping is realizable.

Combining both steps yields
$\mathcal{S}_{\mathrm{MHA}}\subseteq
 \mathcal{S}_{\mathrm{cDAM}}\subseteq
 \mathcal{S}_{\mathrm{uDAM}}$.
\end{proof}


% --------------------------------------------------------
%  Proof of Corollary~\ref{cor:approx-consequence}
% --------------------------------------------------------
\subsection{Proof of Corollary~\ref{cor:approx-consequence}}
\label{app:proof-approx-consequence}

\begin{proof}
Let $\Phi(S):=\sup_{X\in\mathcal{X}}\|S(X)-S^\star(X)\|_{\mathcal{Y}}$.
For any $\mathcal{S}_1\subseteq\mathcal{S}_2$, every feasible point
of $\mathcal{S}_1$ is also feasible in $\mathcal{S}_2$, so
$\inf_{S\in\mathcal{S}_2}\Phi(S)\le\inf_{S\in\mathcal{S}_1}\Phi(S)$.
Applying this monotonicity twice to the hierarchy in
Proposition~\ref{prop:function-class-hierarchy} yields
\[
\varepsilon(\mathcal{S}_{\mathrm{uDAM}};S^\star)
\le
\varepsilon(\mathcal{S}_{\mathrm{cDAM}};S^\star)
\le
\varepsilon(\mathcal{S}_{\mathrm{MHA}};S^\star).
\qedhere
\]
\end{proof}


% --------------------------------------------------------
%  Proof of Proposition~\ref{prop:metric-parameter-complexity}
% --------------------------------------------------------
\subsection{Proof of Proposition~\ref{prop:metric-parameter-complexity}}
\label{app:proof-metric-parameter-complexity}

\begin{proof}
\textbf{Unconstrained CHM.}
There are $h^2$ ordered pairs $(i,j)$, each block
$M_{i,j}\in\mathbb{R}^{d_h\times d_h}$ containing $d_h^2$ scalar
parameters.  Total: $h^2d_h^2=O(h^2d_h^2)$.

\textbf{Constrained DAMCHA.}
(i)~\emph{Diagonal blocks via $f_\theta$}: $h$ blocks of size
$d_h\times d_h$, contributing $hd_h^2$ parameters.
(ii)~\emph{Off-diagonal coefficients}: For each ordered off-diagonal
pair $(i,j)$ with $i\neq j$ (there are $h(h-1)$ such pairs),
there are $h$ scalar coefficients $\alpha_1^{(i,j)},\ldots,\alpha_h^{(i,j)}$,
contributing $h\cdot h(h-1)=h^2(h-1)$ parameters in total.
Grand total: $hd_h^2+h^2(h-1)=O(hd_h^2+h^3)$.

In typical architectures $d_h\gg h$ (e.g.\ $d_h=64$, $h=8$), so
the dominant term is $hd_h^2$ rather than $h^3$, confirming
substantial savings over $h^2d_h^2$.
\end{proof}
